# Supplementary material for: Short Non-Binary Low-Density Parity-Check Codes for Phase Noise Channels
Source: arXiv:1908.02816 source file (2019-08-07)
Supplement: Supplementary file 1 [file appendix.tex]

\section{Mapping of Field Elements to Modulation Symbols}
\label{ch:mapping}
The mappings between field elements and \ac{PSK} symbols are presented in Table \ref{tab:mapping8} and Table \ref{tab:mapping16} for 8-\ac{PSK} and 16-\ac{PSK} respectively.

\begin{table}[th]
	\centering
	\caption{Mapping between field elements, their binary representation and modulation symbols with $m=8$. The primitive polynomial for $\gf{8}$ is $1+\mathrm x+\mathrm x^3$.}\label{tab:mapping8}
	\begin{tabular}{c|c|c}  
		\toprule
		$\gf{8}$ element & Binary label & $8$-PSK symbol\\
		\midrule		
		$0$ & $000$ & $0$ \\
		$\alpha^0$ &$001$ & $e^{j \pi/4}$\\	
		$\alpha^1$ &$010$  & $e^{j 3\pi/4}$	\\	
		$\alpha^2$ &$100$  & $e^{j 7\pi/4}$\\	
		$\alpha^3$& $011$  & $e^{j \pi/2}$\\	
		$\alpha^4$&	$110$  & $e^{j \pi}$\\				     	
		$\alpha^5$& $111$  & $e^{j 5\pi/4}$\\	
		$\alpha^6$ & $101$  & $e^{j 3\pi/2}$\\  
		\bottomrule 					
	\end{tabular}
\end{table}

\begin{table}[h]
	\centering
	\caption{Mapping between field elements, their binary representation and modulation symbols with $m=16$. The primitive polynomial for $\gf{16}$ is $1+\mathrm x+\mathrm x^4$.}\label{tab:mapping16}
	\begin{tabular}{c|c|c}  
		\toprule
		$\gf{16}$ element & Binary label & $16$-PSK symbol\\
		\midrule		
		$0$ 			& $0000$ & $0$ \\
		$\alpha^0	$ 	& $0001$ & $e^{j \pi/8}$ \\
		$\alpha^1	$ 	& $0010$ & $e^{j 3\pi/8}$ \\
		$\alpha^2	$ 	& $0100$ & $e^{j 7\pi/8}$ \\
		$\alpha^3	$	& $1000$ & $e^{j 15\pi/8}$ \\
		$\alpha^4	$	& $0011$ & $e^{j \pi/4}$ \\ 
		$\alpha^5	$	& $0110$ & $e^{j \pi/2}$ \\
		$\alpha^6	$ 	& $1100$ & $e^{j\pi}$ \\
		$\alpha^7	$ 	& $1011$ & $e^{j 13\pi/8}$ \\
		$\alpha^8	$ 	& $0101$ & $e^{j 3\pi/4}$ \\
		$\alpha^9	$ 	& $1010$ & $e^{j 3\pi/4}$ \\
		$\alpha^{10}$ 	& $0111$ & $e^{j 5\pi/8}$ \\
		$\alpha^{11}$	& $1110$ & $e^{j 11\pi/8}$ \\
		$\alpha^{12}$	& $1111$ & $e^{j 5\pi/4}$ \\
		$\alpha^{13}$	& $1101$ & $e^{j 9\pi/8}$ \\
		$\alpha^{14}$ 	& $1001$ & $e^{j 7\pi/4}$ \\
		\bottomrule 					
	\end{tabular}
\end{table}
